# Supplementary material for: On Fairness and Calibration
Source: arXiv:1709.02012 source file (2017-11-03)
Supplement: Supplementary file 1 [file feasibility_proofs.tex]

\section{Proof of \autoref{thm:feasibility} (Feasibility)}
\label{sec:detailed-feasibility}

We will now give a detailed proof of \autoref{thm:feasibility}, which
is restated below:
\newtheorem*{thm:feasibility}{Theorem \ref{thm:feasibility} (Restated)}
\begin{thm:feasibility}
  Let $h_1$ and $h_2$ be (approximately) calibrated classifiers
  for groups $G_1$ and $G_2$, respectively. If $\fairconst{h_2}{2} < \fairconst{h_1}{1} \leq
  \argmax_{h^*_2 \in \mathcal{H}^*_2} \fairconst{h^*_2}{2}$, where
  $\mathcal{H}^*_2$ is the set of calibrated classifiers for group $G_2$,
  then there exists some classifier $\fair h_2$ for group $G_2$ with
  $\calib{\fair h_2} \leq \calib{h_2}$ and $\fairconst{h_1}{1} = \fairconst{\fair h_2}{2}$.
\end{thm:feasibility}
As stated in \autoref{sec:feasibility}, we will use \autoref{alg:method} in
a proof by construction.
This involves constructing $\fair h_2$, a classifier which replaces some predictions
of $h_2$ with predictions from the trivial classifier $h^\triv_2$:
\begin{equation*}
  \fair{h}_2(\x) = (1 - B) h_2(\x) + B h^\triv_2(\x).
  \tag{\ref{eqn:fair_classifier} restated}
\end{equation*}
where $B$ is a Bernoulli variable with expectation $\alpha$.
We will show in \autoref{thm:calibration} and \autoref{crly:exists_equal_cost}
that the resultant classifier meets the (approximate) calibration and no-disparity
conditions of \methodname{}.

%\paragraph{Ensuring No Disparity.}
%Intuitively, it is possible to achieve the disparity constraint because
%the interpolated classifier $\fair h_2$ can achieve any
%cost in the interval $\left[ \fairconst{h_2}{2}, \fairconst{h^\triv_2}{2} \right]$.

%\paragraph{Ensuring Calibration.}

%Intuitively, \autoref{alg:method} maintains calibration because we are randomly
%sampling between two calibrated classifiers. We have that $\calib{h_2}$ is
%small, and it is seen through \autoref{def:calibration} that $h_t^\triv$ is
%perfectly calibrated. Therefore, $\fair h_2$ should also be approximately calibrated.
%More formally,

%
\begin{lemma}
  Given $\fair h_2$, which is the classifier derived from \eqref{eqn:fair_classifier},
  we have that $\calib{\fair h_2} \leq \left( 1 - \alpha \right) \calib{h_2}$, where
  $\alpha \in [0, 1]$ is the interpolation parameter in \eqref{eqn:fair_classifier}.
  \label{thm:calibration}
\end{lemma}
\begin{proof}
  %Again, let $h_t$ be a classifier for group $G_t$, and let $h^\triv_t$ be the
  %trivial classifier for $G_t$.
  %Finally, we assume that $\fair h_t$ randomizes between the two classifiers, i.e.
  %\[
    %\fair h_t(\x) = (1-B) h_t(\x) + B h^\triv_t(\x)
  %\]
  %where $B$ is a Bernoulli random variable with parameter $\alpha$.
  We can calculate the calibration of $\fair h_2(\x)$ as follows:
  \begin{align*}
    \calib{\fair h_2}
    &= \mathop{\ev}_{B, G_2} \Bigl\lvert \Pr_{G_2} \bigl[ y\!=\!1 \mid \fair
    h_2(\x)\!=\!p \bigr] - p \Bigr\rvert
    \\
    &= \int_{0}^1 \sum_{b=0}^1 \Bigl\lvert \Pr_{G_2} \bigl[ y\!=\!1 \mid \fair
    h_2(\x) \!=\!p \bigr] - p \Bigr\rvert
    %\\ &\phantom{=} \times
    \Pr_{G_2} \bigl[ \fair h_2(\x)\!=\!p, B\!=\!b \bigr] dp
    \\
    &= \int_{0}^1 \Biggl( \Bigl\lvert \Pr_{G_2} \bigl[ y\!=\!1 \mid h_2(\x)
    \!=\!p \bigr] - p \Bigr\rvert \Pr_{G_2} \bigl[ h_2(\x)\!=\!p, B\!=\!1 \bigr]
    %\\ &\phantom{=}
    + \Bigl\lvert \Pr_{G_2} \bigl[ y\!=\!1 \mid h^\triv_2(\x) \!=\!p
    \bigr] - p \Bigr\rvert \Pr_{G_2} \bigl[ h^\triv_2(\x)\!=\!p, B\!=\!0 \bigr] \Biggr) dp
    \\
    &= \int_{0}^1 \Biggl( \alpha \Bigl\lvert \Pr_{G_2} \bigl[ y\!=\!1 \mid
    h_2(\x) \!=\!p \bigr] - p \Bigr\rvert \Pr_{G_2} \bigl[ h_2(\x)\!=\!p \bigr]
    %\\ &\phantom{=}
    +  \bigl( 1 \! - \! \alpha \bigr) \Bigl\lvert \Pr_{G_2}
    \bigl[ y\!=\!1 \mid h^\triv_2(\x) \!=\!p \bigr] - p \Bigr\rvert \Pr_{G_2}
    \bigl[ h^\triv_2(\x)\!=\!p \bigr] \Biggr) dp
    \\
    &= (1-\alpha) \calib{h_2} + \alpha \calib{h^\triv_2}.
  \end{align*}
  Because the trivial classifier is perfectly calibrated, we have that $\calib{\fair h_t} = (1 - \alpha) \calib{h_t}$.
\end{proof}
By this theorem, $\calib{\fair h_2}$ is no greater than $\calib{h_2}$.
Therefore, if we can assume that our original classifier is well calibrated, then
our derived classifier will also be well calibrated.
\begin{lemma} \label{lma:interpolation}
  Let $\fair h_2$ be the classifier derived from \eqref{eqn:fair_classifier}
  with interpolation parameter $\alpha \in [0, 1]$.
  The cost of $\fair h_2$ is given by
  \[
    \fairconst{\fair h_2}{2} = (1 - \alpha) \fairconst{h_2}{2} + \alpha \fairconst{h^\triv_2}{2}
  \]
\end{lemma}
\begin{proof}
  We assume that $\fairconstname$ is a cost function which follows the form of \eqref{eqn:cost_general} ---
  i.e.
  \[ \fairconst{h_t}{t} = a_t \fp{h_t} + b_t \fn{h_t} \]
  for some non-negative constants $a_t$ and $b_t$.
  The cost of $\fair h_2$ can be calculated using linearity of expectation:
  \begin{align*}
    \fairconst{\fair h_2}{2} &= a_2 \fp{\fair h_2} + b_2 \fn{\fair h_2}
    \\&= a_2 \ev_{G_2} \left[ 1 -  \fair h_2(\x) \mid y\!=\!1 \right] + b_2 \ev_{G_2} \left[ \fair h_2(\x) \mid y\!=\!0 \right]
    \\&= a_2 \ev_{B,G_2} \left[ 1 - \left[ (1-B) h_2(\x) + B h^\triv_2(\x) \right] \mid y\!=\!1 \right]
    %\\&\phantom{=} \:
    + b_2 \ev_{B,G_2} \left[ \left[ (1-B) h_2(\x) + B h^\triv_2(\x) \right] \mid y\!=\!0 \right]
    \\&=                a_2 \ev_{B,G_2} \left[ (1-B) \left( 1 - h_2(\x) \right) \mid y\!=\!1 \right]
    %\\&\phantom{=} \:
    + a_2 \ev_{B,G_2} \left[ B \left( 1 -  h^\triv_2(\x) \right) \mid y\!=\!1 \right]
    \\&\phantom{=} \:
    + b_2 \ev_{B,G_2} \left[ (1-B) h_2(\x) \mid y\!=\!0 \right]
    %\\&\phantom{=} \:
    + b_2 \ev_{B,G_2} \left[ B h^\triv_2(\x) \mid y\!=\!0 \right]
    \\&=                a_2 \ev_{B} \left[ 1-B \right] \ev_{G_2} \left[ 1 - h_2(\x) \mid y\!=\!1 \right]
    %\\&\phantom{=} \:
    + a_2 \ev_{B} \left[ B \right]   \ev_{G_2} \left[ 1 -  h^\triv_2(\x) \mid y\!=\!1 \right]
    \\&\phantom{=} \:
    + b_2 \ev_{B} \left[ 1-B \right] \ev_{G_2} \left[ h_2(\x) \mid y\!=\!0 \right]
    %\\&\phantom{=} \:
    + b_2 \ev_{B} \left[ B \right]   \ev_{G_2} \left[ h^\triv_2(\x) \mid y\!=\!0 \right]
    \\&= a_2 (1-\alpha) \fp{h_2} + b_2 (1-\alpha) \fn{h_2}
    %\\&\phantom{=} \:
    + a_2 (\alpha) \fp{h^\triv_2} + b_2 (\alpha) \fn{h^\triv_2}
    \\&= (1 - \alpha) \fairconst{h_2}{2} + \alpha \fairconst{h^\triv_2}{2}.
  \end{align*}
\end{proof}
\begin{corollary}
  \label{crly:exists_equal_cost}
  Assume that $\fairconst{h_1}{1} \in \left[ \fairconst{h_2}{2}, \fairconst{h^\triv_2}{2} \right]$.
  If we construct $\fair h_2$ such that
  $
    \alpha = \frac{\fairconst{h_1}{1} - \fairconst{h_2}{2}}{\fairconst{h^\triv_2}{2} - \fairconst{h_2}{2}},
  $
  then $\dispar{h_1}{1}{\fair h_2}{2} = 0$.
\end{corollary}
Finally, note that \autoref{lma:trivial} that $\fairconst{h_2}{2}$ has the highest cost of any
calibrated classifier for group $G_2$.
\begin{lemma}
  For any cost function $\fairconstname$ that follows the form of
  \eqref{eqn:cost_general}, the trivial classifier $h^\triv_t$ is the calibrated
  classifier for $G_t$ with maximum cost.
  \label{lma:trivial}
\end{lemma}
\begin{proof}
  %Let $r_t = \Pr_{G_t} \left[ y = 1 \right]$ be the base rate for group $G_t$.
  %It can be seen that for any calibrated classifier that $\ev_{G_t} \left[ h(\x) \right] = r_t$.
  Again, let $\fairconstname$ be a cost function:
  $$\fairconst{h}{t} = a_t \fp{h_t} + b_t \fn{h_t}.$$
  Using \eqref{eqn:fp_exact} and \eqref{eqn:fn_exact}, we have that, for every classifier $h^*_t$
  that is perfectly calibrated for group $G_t$,
  \begin{align*}
    \fairconst{h^*_t}{t} &= a_t \fp{h^*_t} + b_t \fn{h^*_t}
    \\&= \left( \frac{a_t}{1 - \mu_t} + \frac{b_t}{\mu_t} \right) \left( \ev_{G_t} \left[ h^*_t(x) \right] - \ev_{G_t} \left[ h^*_t(x)^2 \right] \right)
    \\&= \left( \frac{a_t}{1 - \mu_t} + \frac{b_t}{\mu_t} \right) \left( \mu_t - \ev_{G_t} \left[ h^*_t(x)^2 \right] \right).
  \end{align*}
  The last equation holds because $\ev_{G_t} \left[ h^*_t(\x) \right] = \mu_t$ for any calibrated
  classifier -- a fact which can easily be derived from \autoref{def:calibration}.

  We would like to find, $h^{\max}_t \in \mathcal{H}^*_t$, the calibrated classifier with the highest weighted cost.
  Because $\left( \frac{a_t}{1 - \mu_t} + \frac{b_t}{\mu_t} \right)$ and $\mu_t$ are non-negative constants, we have
  \begin{align*}
    h^{\max}_t &= \argmax_{h \in \mathcal{H}^*_t} \Bigl[ \left( \frac{a_t}{1 - \mu_t} + \frac{b_t}{\mu_t} \right) \left( \mu_t - \ev_{G_t} \left[ h(x)^2 \right] \right) \Bigr]
    \\&= \argmax_{h \in \mathcal{H}^*_t} \Bigl[ - \ev_{G_t} \left[ h(x)^2 \right] \Bigr]
    \\&= \argmin_{h \in \mathcal{H}^*_t} \Bigl[ \ev_{G_t} \left[ h(x)^2 \right] \Bigr]
    \\&= \argmin_{h \in \mathcal{H}^*_t} \Bigl[ \ev_{G_t} \left[ h(x)^2 \right] - \mu_t^2 \Bigr]
    \\&= \argmin_{h \in \mathcal{H}^*_t} \Bigl[ \ev_{G_t} \left[ h(x)^2 \right] - \ev_{G_t} \left[ h(x) \right]^2 \Bigr]
  \end{align*}
  Thus, the calibrated classifier with minimum variance will have the highest cost. This translates to
  a classifier that outputs the same probability for every sample. By the calibration constraint, this
  constant must be equal to $\mu_t$, so therefore this classifier must be the trivial classifier $h^\triv_t$ --- i.e.
  for all $\x$
  \[ h^{\max}_t \left( \x \right) = h^\triv_t \left( \x \right) = \mu_t. \]
\end{proof}
Putting the results of Lemmas~\ref{thm:calibration}, \ref{thm:interpolation}, and \ref{lma:trivial}
together
completes the proof for \autoref{thm:feasibility}.
%
%
%
%\kilian{The problem with the section up to here is that you lost the
%connection to the application.  Can you add 1-2 sentences  after each  theorem
%/ Corollary   and explain what it means, ideally relating it back to the
%running example?}
%
